# Supplementary material for: A Closed-Loop Perception, Decision-Making and Reasoning Mechanism for Human-Like Navigation
Source: arXiv:2207.11901 source file (2022-07-25)
Supplement: Supplementary file 1 [file Appendix.tex]

\section{Appendix}
\subsection{Implementation details}      
The observation is defined as $o_{t}=[o_{t}^{L};o_{t}^{P};o_{t}^{V}]$, which is a 184-dimensional vector. The action is defined as $a_{t}=[v_{t};w_{t}]$, representing the Forward and Angular velocity respectively. The reward function of the all comparison algorithms is set identically. All models are implemented using PyTorch. We use optimizer Adam with a learning rate of 1e-3 in Dual-VAE Demonstration learning and 3e-5 in Dual-RL Interaction learning.

\subsection{Navigation scene}
We train the algorithm using two simple scenarios, one of which is a static scene and the other is a dynamic scene. The dynamic scene has a large number of dynamic obstacles that wander randomly, and these obstacles vary in size and shape. For testing, we designed two test benchmarks(few-shot scene and zero-shot scene). Each benchmark consists of 8 challenging navigation scenarios, including mazes, roadblocks, traffic intersections. The eight scenarios in the Few-shot-scene benchmark are relatively simple and similar to the training environment. To design zero-shot scene, we impose some specific changes(density, speed, shape change and so on) to each scene from the few-shot scene and also add some noise to the sensor. Therefore, all eight scenarios in the zero-shot-scene benchmark are quite novel to the agent. The purpose is to test the generalization and robustness of the algorithm under new scenarios with dissimilar distributions.

\subsection{Real-world experiment}
We used a wheeled robot(Turtlebot3) to conduct a navigation experiment in an office building(about 800$m^{2}$) with moving pedestrians. The robot is equipped with a 16-line 3D-LIDAR(Velodyne-16) and a depth camera(Real-Sense D435) to obtain the distance of surrounding obstacles and the robot's own position. In addition, to achieve fully autonomous navigation, the robot also mounts an edge computing device(NVIDIA Jetson AGX Xavier). The action commands for the robot is generated by Xavier installed with Ubuntu 18.04 and ROS Melodic. All calculation processes are performed online.
